# Supplementary material for: GAIA-1: A Generative World Model for Autonomous Driving
Source: arXiv:2309.17080 source file (2023-09-29)
Supplement: Supplementary file 1 [file Appendix.tex]

\clearpage
\appendix

\section{Full Model Architecture}
[Give all the details about the shape of the network]

[Give all the training hyperparameters]

\subsection{Image Tokenizer}
\label{appendix:image-tokenizer}

\subsection{World Model}
\label{appendix:world-model}

\subsection{Video Decoder}
\label{appendix:video-decoder}
